# Supplementary material for: Connecting Parameter Magnitudes and Hessian Eigenspaces at Scale using Sketched Methods
Source: arXiv:2504.14701 source file (2025-04-20)
Supplement: Supplementary file 1 [file bibliography.tex]

% !TeX root = ../main.tex

\bibliographystyle{unsrtnat}
\bibliography{appendix/bibliography}
