# Supplementary material for: Connecting Parameter Magnitudes and Hessian Eigenspaces at Scale using Sketched Methods
Source: arXiv:2504.14701 source file (2025-04-20)
Supplement: Supplementary file 2 [file broader_impact.tex]

This paper presents work whose goal is to advance the field of Machine Learning. There are many potential societal consequences of our work, none of which we feel must be specifically highlighted here.
